# Supplementary material for: Solidification of the Lennard-Jones fluid near the wall in thermohydrodynamic lubrication
Source: arXiv:1902.03744 source file (2019-02-11)
Supplement: Supplementary file 1 [file supplement.pdf]

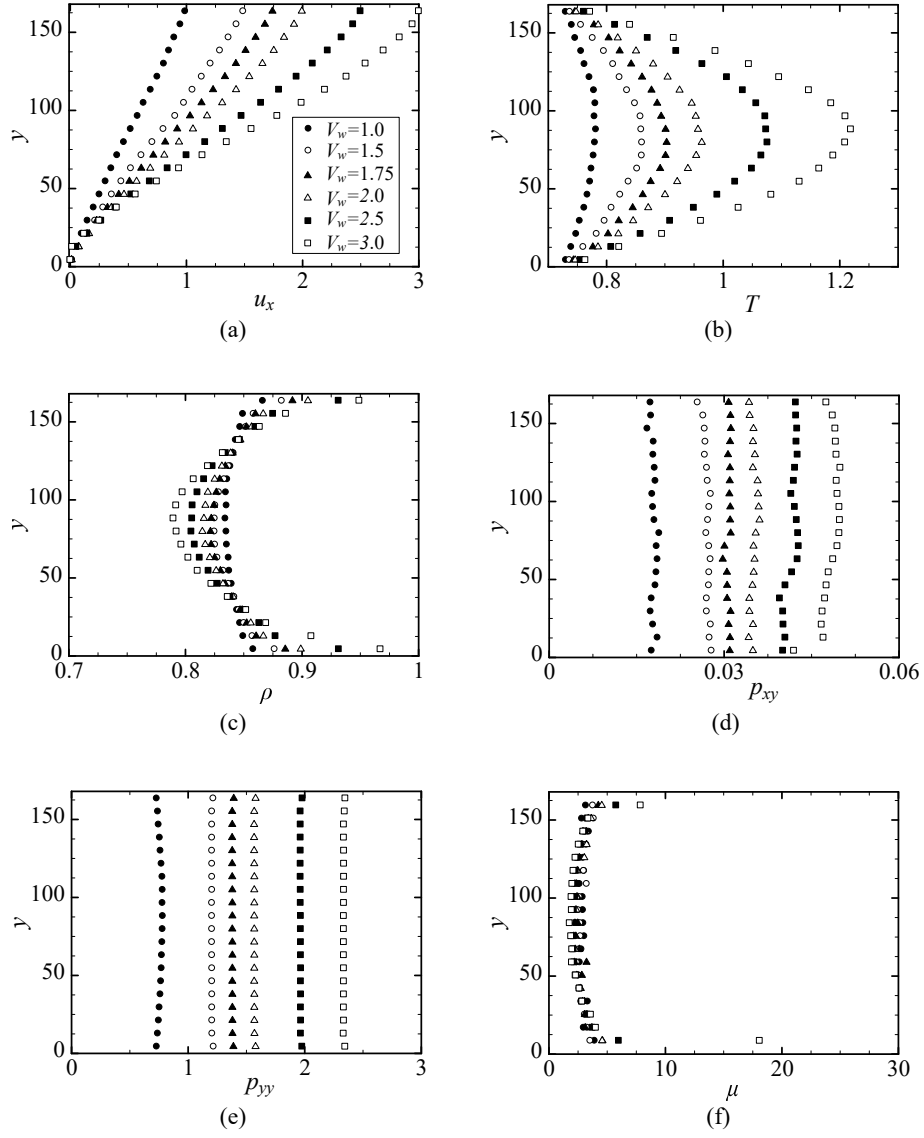

FIG. 1: The spatial distributions of the macroscopic quantities, i.e., (a) velocity  $u_x$ , (b) temperature  $T$ , (c) density  $\rho$ , (d) shear stress  $p_{xy}$ , (e) normal stress  $p_{yy}$ , and (f) local viscosity  $\mu$ , for different wall velocities  $V_w$  in the channel where  $H = 168$

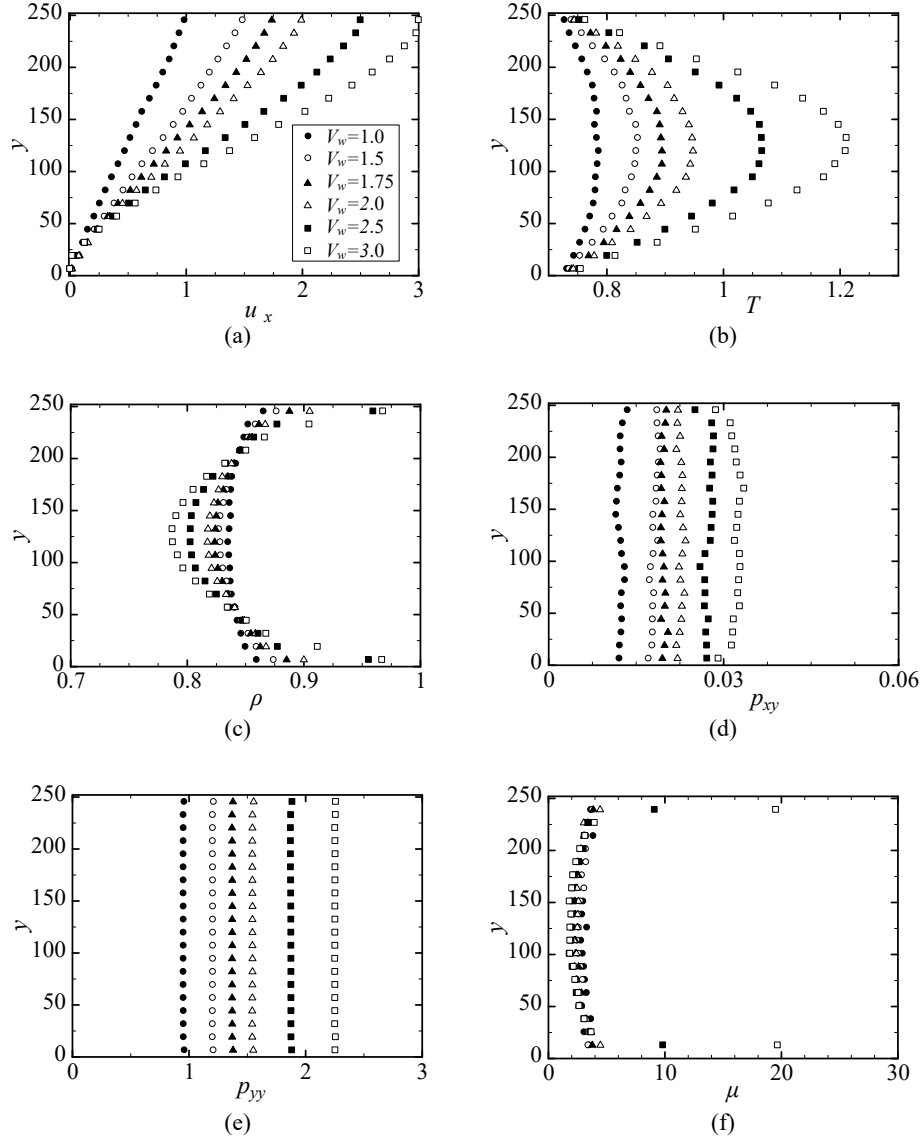

FIG. 2: The spatial distributions of the macroscopic quantities, i.e., (a) velocity  $u_x$ , (b) temperature  $T$ , (c) density  $\rho$ , (d) shear stress  $p_{xy}$ , (e) normal stress  $p_{yy}$ , and (f) local viscosity  $\mu$ , for different wall velocities  $V_w$  in the channel where  $H = 252$

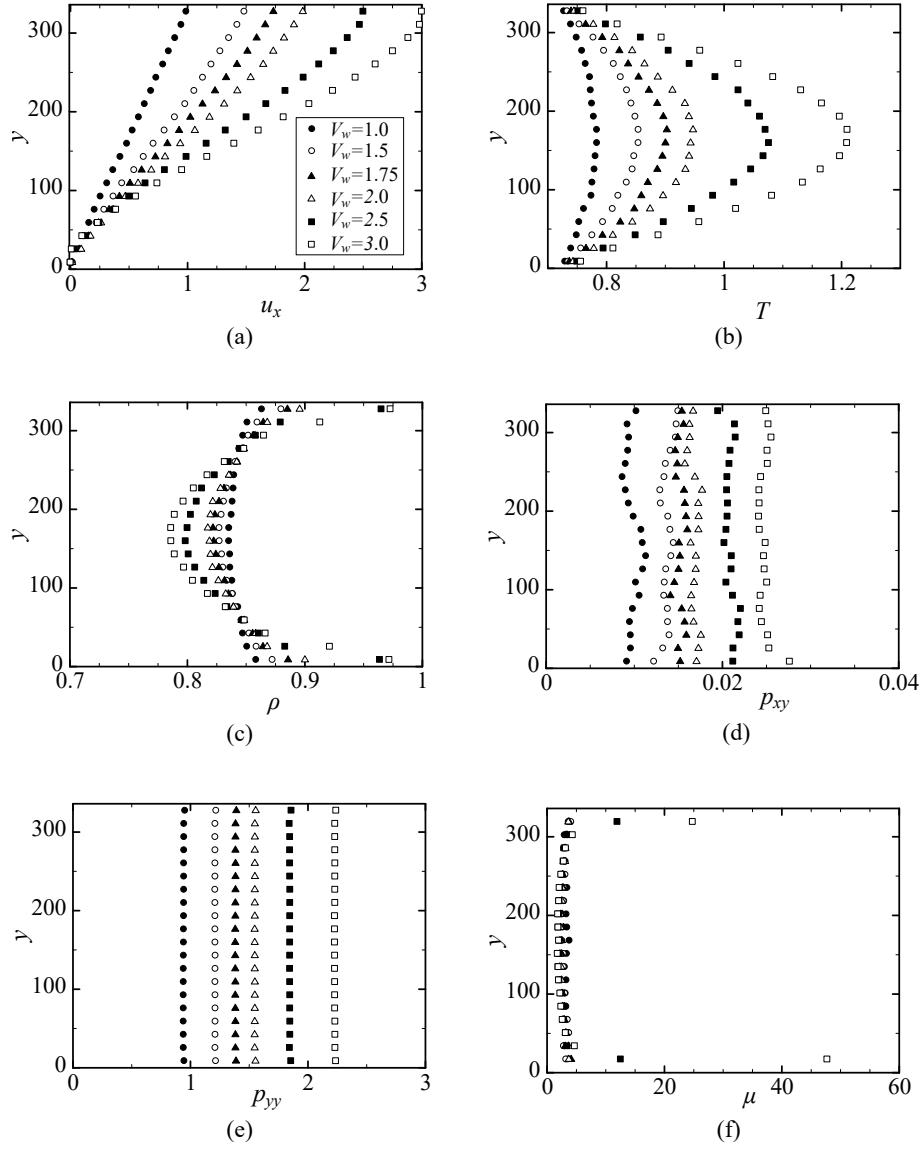

FIG. 3: The spatial distributions of the macroscopic quantities, i.e., (a) velocity  $u_x$ , (b) temperature  $T$ , (c) density  $\rho$ , (d) shear stress  $p_{xy}$ , (e) normal stress  $p_{yy}$ , and (f) local viscosity  $\mu$ , for different wall velocities  $V_w$  in the channel where  $H = 336$

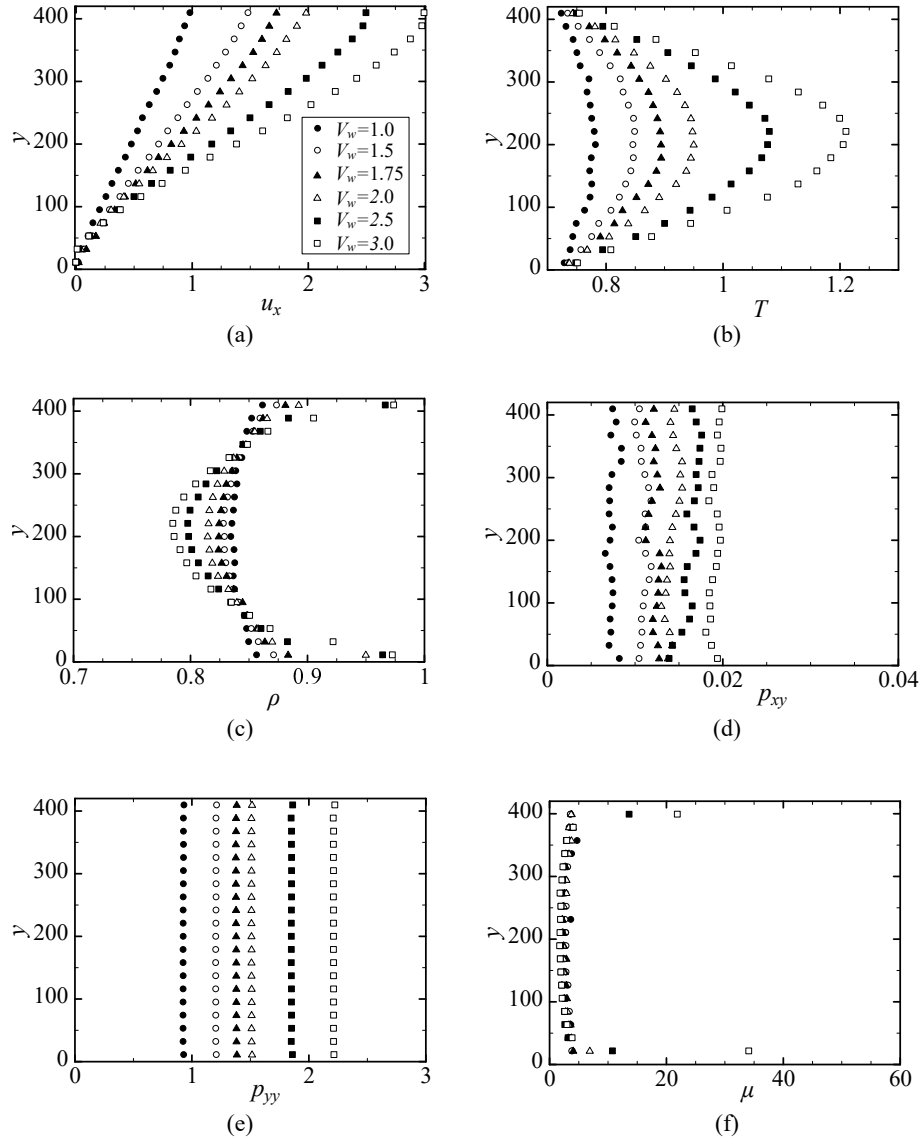

FIG. 4: The spatial distributions of the macroscopic quantities, i.e., (a) velocity  $u_x$ , (b) temperature  $T$ , (c) density  $\rho$ , (d) shear stress  $p_{xy}$ , (e) normal stress  $p_{yy}$ , and (f) local viscosity  $\mu$ , for different wall velocities  $V_w$  in the channel where  $H = 420$

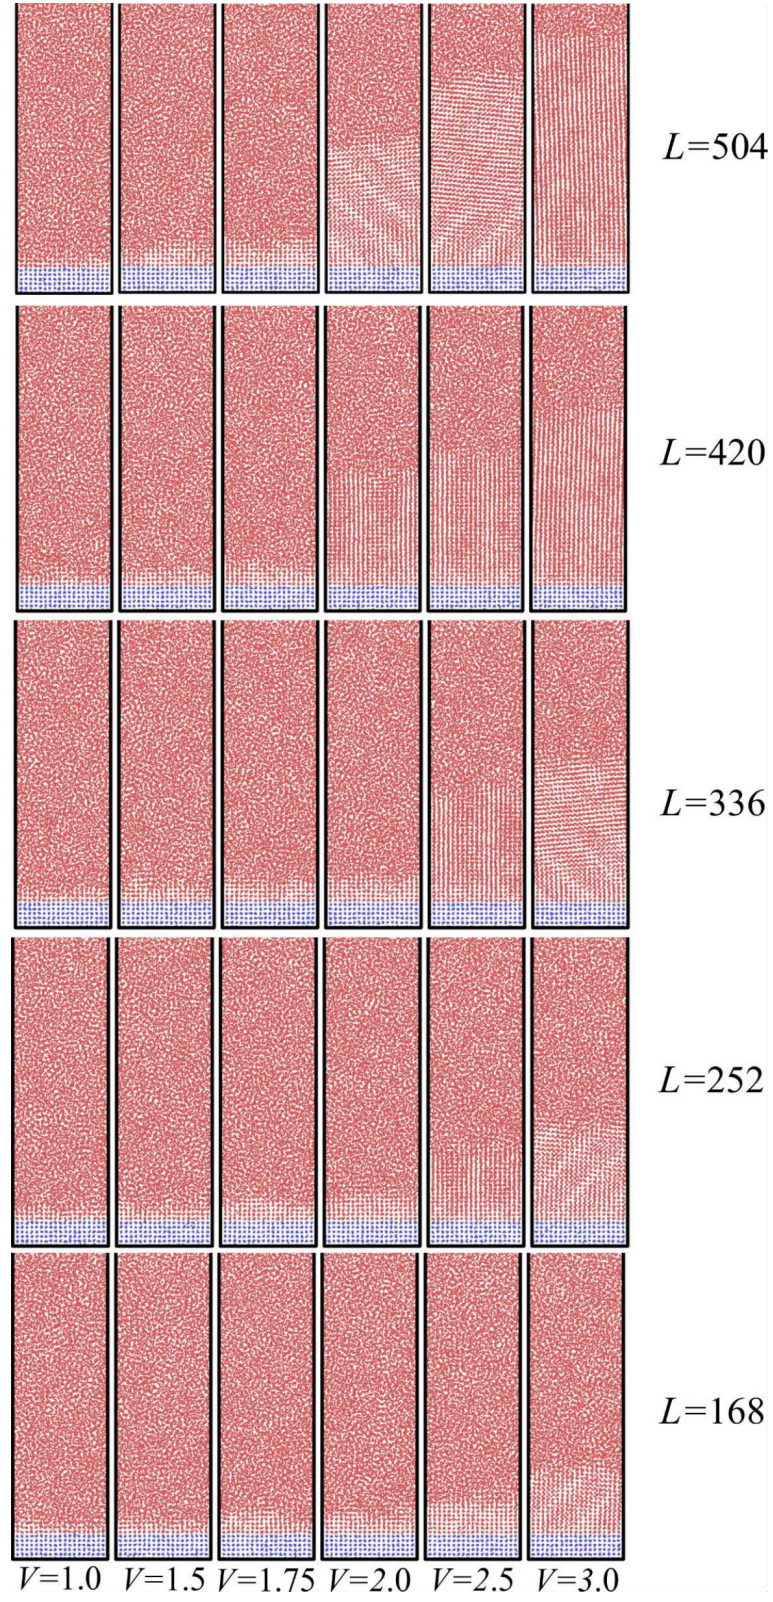

FIG. 5: Snapshots of the LJ molecules in the vicinity of wall ( $0 < y < 60$ ) and the wall molecules for different channel widths  $L$  and wall speeds  $V$ .
